# Supplementary material for: High-Rate Phase Association with Travel Time Neural Fields
Source: arXiv:2307.07572 source file (2024-12-12)
Supplement: Supplementary file 1 [file SI.pdf]

# Supplementary information: High-Rate Phase Association with Travel Time Neural Fields

Cheng Shi[1], Giulio Poggiali[2], Chris Marone[2,5], Maarten V. de Hoop[3,*] and Ivan Dokmanić[1,4,*]
[1]Departement of Mathematics and Computer Science, University of Basel,
[2]Department of Earth Sciences, La Sapienza Università di Roma,
[3]Simons Chair in Computational and Applied Mathematics and Earth Science, Rice University,
[4]Department of ECE, University of Illinois at Urbana–Champaign,
[5]Department of Geosciences, Pennsylvania State University
[*]To whom correspondence should be addressed; E-mail: ivan.dokmanic@unibas.ch, mvd2@rice.edu

December 12, 2024

**Contents of this file**

1. Text: Section S1 to S8
2. Figures SF1 to SF15

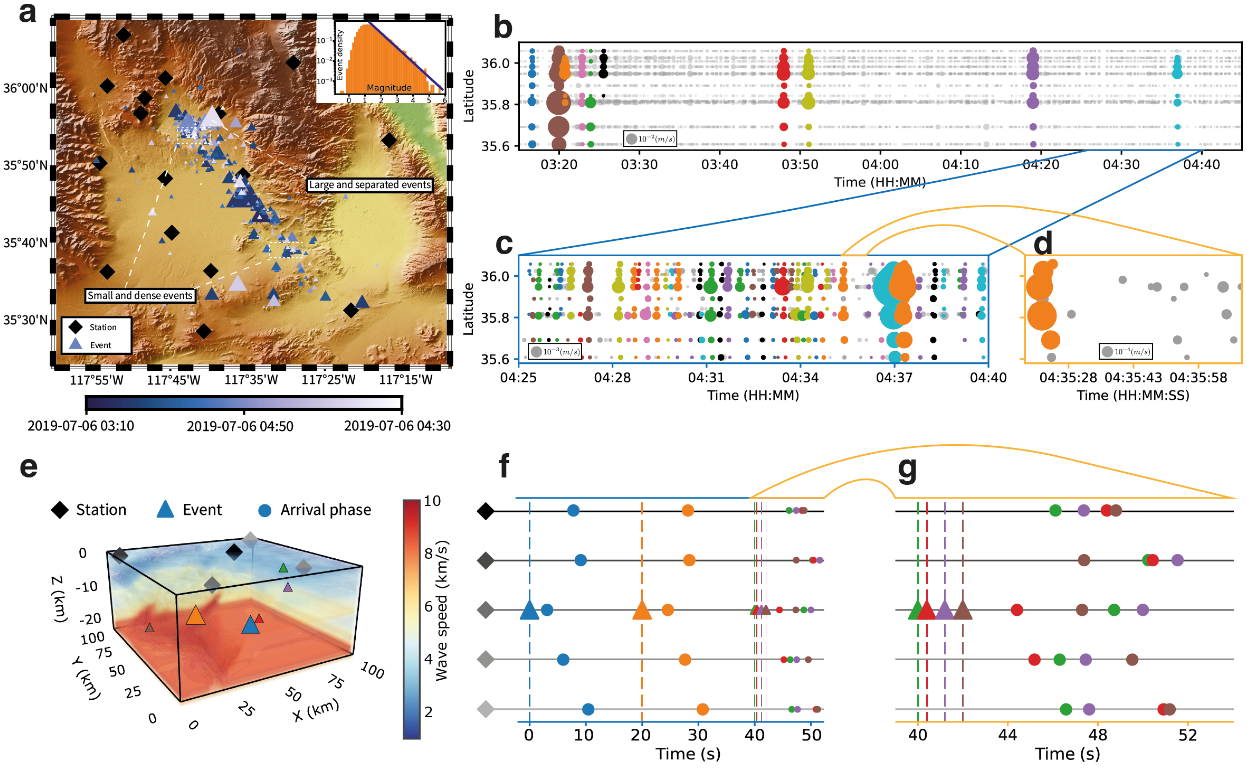


Figure SF1: Seismic events shown at different spatiotemporal scales. Panel **a**: Data from Ridgecrest CA, recorded on July 6, 2019, between 04:10 and 04:30, showing both large, isolated events and small, clustered ones. Triangle sizes represent earthquake magnitudes; color represents arrival times. Inset shows the frequency magnitude distribution, where the slope represents the Gutenberg-Richter $b$ value. Panel **b**: low-rate large magnitude events, which are easy to associate. Each trace corresponds to a record from one station shown at its latitude on the y-axis. Dot diameters are proportional to recorded peak ground velocity (PGV) [1] and color represents the association, that is, waveforms from a common seismic source. Gray dots in **c, d** indicate wave arrivals that are not associated and therefore represent unidentified earthquakes [2]. Large magnitude arrivals in panel **b** are simple to associate. Panel **c** illustrates a time interval, at finer scale, that is more challenging for association but nonetheless successful as the arrival time fluctuations due to the henetrogeneity in wavespeed are still small compared to the intermittancy (rate) of events. At yet a finer time scale and shorter interval in panel **d** identification and association becomes a challenge and has, by traditional techniques, been unresolved. This intermittancy originates from yet smaller earthquakes in accordance with the Gutenberg-Richter law. On the one hand, the detection of ever smaller events is challenging due to “background” noise; on the other hand, the implied increasing rate poses the challenge of association due to wavespeed uncertainties and changes with time due to earthquake fault motion and fracturing. It is the latter that we address and illustrate in panels **e**, **f**, and **g**. Here, we demonstrate this using a synthetic wave speed model, the SEG/EAGE 3-D overthrust, with congruent spatial dimensions. Blue and orange triangles indicate two earthquakes occurring 20 seconds apart, with easily associated arrivals (panel **g**). The remaining four smaller triangles indicate events that all occur within 2 seconds, presenting a significantly harder association challenge where the ordinal number of arrival carries no significance (panel **g**). We note that for greater fracturing and stronger wave speed fluctuations the association challenge becomes apparent for even larger magnitude earthquakes.

# S1 Confusion factor

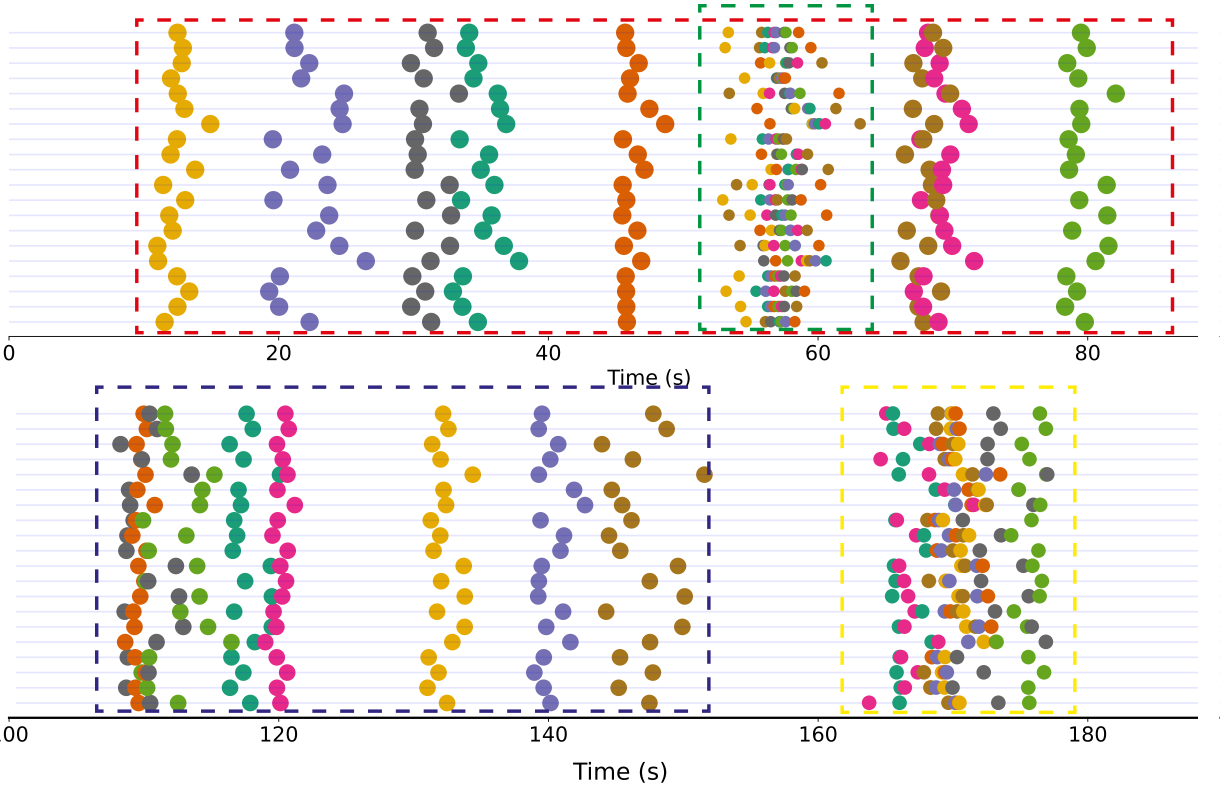


Figure SF2: Phase association for different arrival rates / confusion factors. Each colored frame contains 8 sources recorded by 20 stations. Each horizontal line represents a stations, with colored circles representing arrivals. CF is confusion factor (Equation SE1) and ACC is association accuracy (Equation SE5). The inner circle color encodes the ground truth association; the outer circle color encodes association computed by HARPA. **Green**: CF $= 0.88$, ACC $= 97.5\%$, $e_l = 0.04$ s; **yellow**: CF $= 0.42$, ACC $= 98.8\%$, $e_l = 0.03$ s; **navy blue**: CF $= 0.05$, ACC $= 100\%$, $e_l = 0.02$ s; **red**: CF $= 0.02$, ACC $= 100\%$, $e_l = 0.03$ s.

The frequency of the event is not the only factor that influences the degree of arrival overlap; other factors, such as the depth of the event and the speed of the wave, also play a role. To better quantify the level of disorder in seismic event arrivals, and to compare the difficulty of joint inference and association problems, we define the *confusion factor* (CF) which ranges from 0 to 1. A value close to 0 indicates that the picks arrive in a similar order across stations and are easy to associate (e.g., red box in Fig. SF2). Conversely, a value close to 1 indicates that the picks arrive in a confused manner (e.g., green box in Fig. SF2). The CF is mathematically defined as follows:

$$\begin{aligned} \mathsf{CF} &= 1 - \max\left\{ \frac{1}{N} \sum_{i=1}^{N} \mathcal{T}\left[ \{ (T_c(s_j; r_i) + \tau_j,\ \tau_j) \}_{j=1}^{M} \right], 0 \right\} \\ &= 1 - \max\left\{ \frac{1}{N} \sum_{i=1}^{N} \mathcal{T}\left[ \{ (t_{i,\alpha^*(j;r_i)}, \tau_j) \}_{j=1}^{M} \right], 0 \right\}, \end{aligned} \qquad \text{(SE1)}$$

where

$$\mathcal{T}\left[ \{ (a_j, b_j) \}_j \right] = \frac{\text{number of concordant pairs} - \text{number of discordant pairs}}{\text{number of pairs}}$$

calculates Kendall's $\tau$ rank correlation coefficient [3]. Succinctly, when the order of the arrivals at a station matches the order of earthquake occurrences, $\mathcal{T}$ yields a value of 1 and $\mathsf{CF} = 0$. This typically occurs during low-rate earthquakes, where the travel time is shorter than the time between the different events. Conversely, when all earthquakes occur almost simultaneously, the order of earthquake occurrence bears no correlation with the order of the phases/picks arriving at the stations. This reduces $\mathcal{T}$ closer to 0, and pushes $\mathsf{CF}$ closer to 1, implying a higher level of confusion (the $\mathsf{CF}$ is always between 0 and 1). When studying regions such as Ridgecrest around the time of the 2019 earthquake, the magnitude cutoff is usually chosen so that the resulting $\mathsf{CF}$ is below 0.1 [4, 2, 5], while the 2014 Chile earthquake has the $\mathsf{CF}$ lower than 0.01. Fig. SF2 shows representative arrival configurations for different values of $\mathsf{CF}$; Fig. SF9 shows results of an exhaustive test of the proposed method at different $\mathsf{CF}$. In S7, we define the accuracy and error metric for the association result.

# S2 Higher frequency event and seismograms

In Fig. 1 of the main text, we generate highly entangled arrivals by advancing or delaying cataloged event and corresponding phases. This approach can also be applied to seismograms. In Fig. SF3, we first select a slice of seismograms from the Ridgecrest 2019 dataset. Phase picking is performed using PhaseNet, and events are associated using Harpa, as shown in the first and second rows of Fig. SF3. For each identified event, we extract the corresponding waveforms and set the remaining noise portions of the waveform to zero (as shown in the third and fourth rows).

Next, using the same strategy employed in Fig. 1 main text, we advance or delay the occurrence times of events by consistently adjusting the arrival times and the corresponding waveform slices for each event. The fifth, sixth, and seventh rows illustrate three cases with frequencies of 0.3 epm, 3 epm, and 30 epm, respectively. Events, along with their P- and S-phases, are plotted on the same time axis. The color of P- and S-phases represents their corresponding event.

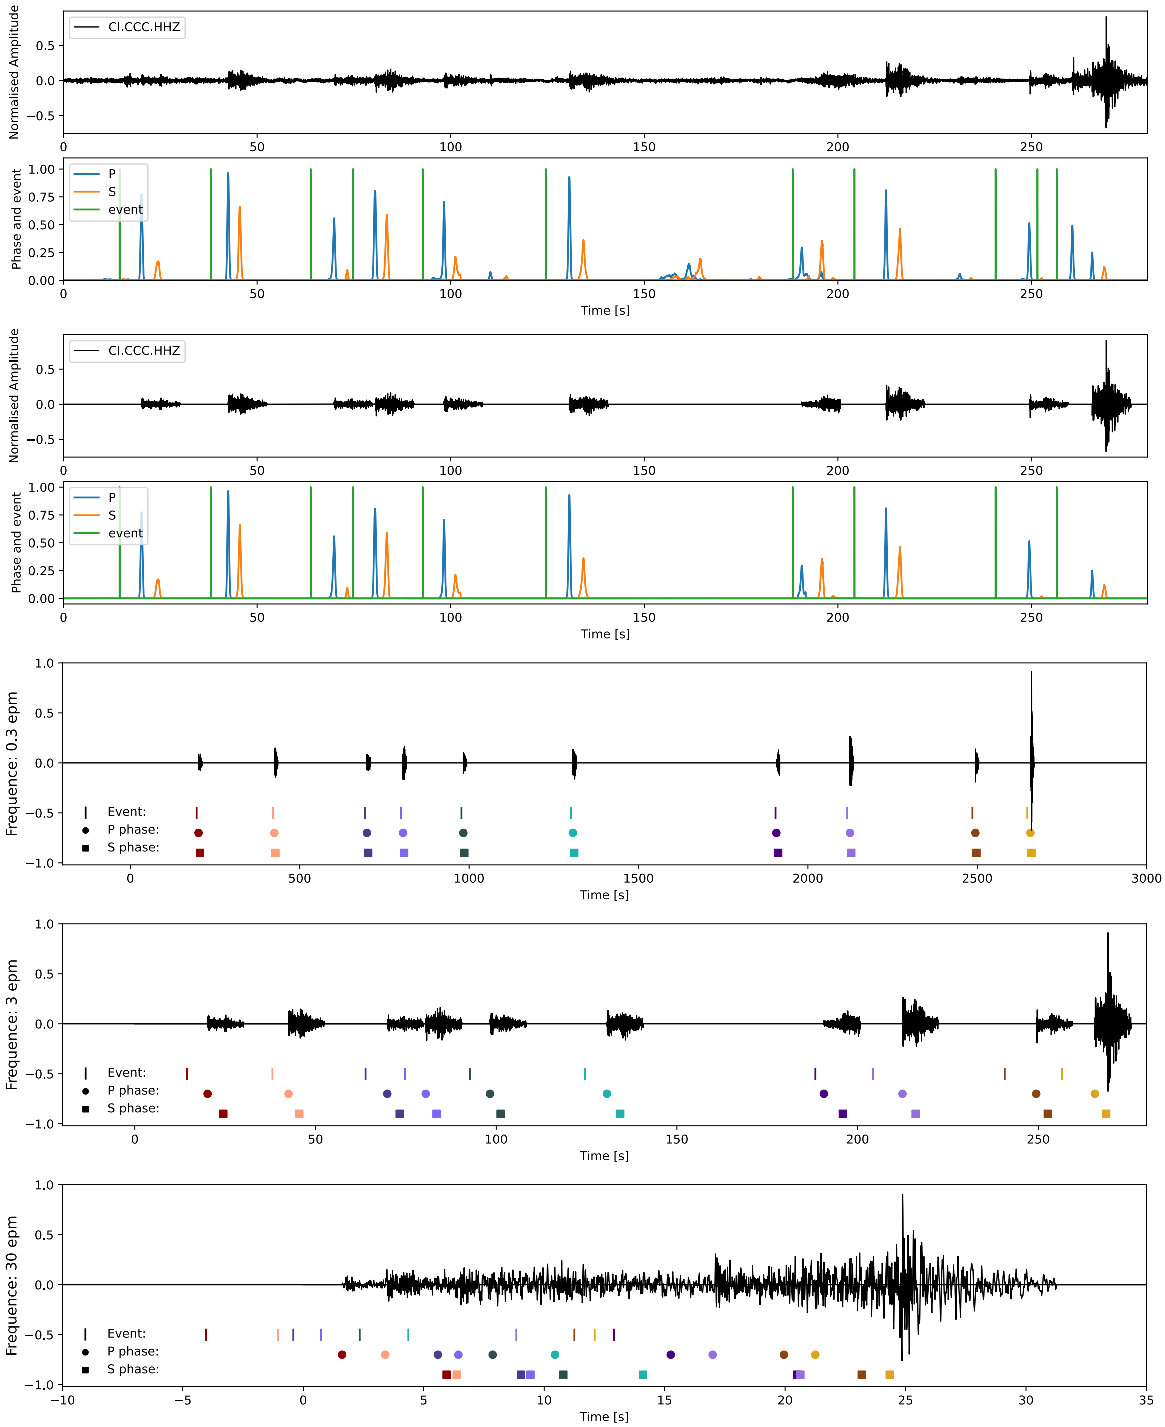


Figure SF3: Seismograms of synthetic high-rate events created with data from Ridgecrest 2019 earthquake. Details in S2.

As shown in the last row of Fig. SF3, the waveforms are highly overlapped at 30 epm. We demonstrate that the current phase-picking algorithm, such as PhaseNet, struggles to accurately pick phases from such overlapped waveforms, as shown in Fig. SF4.

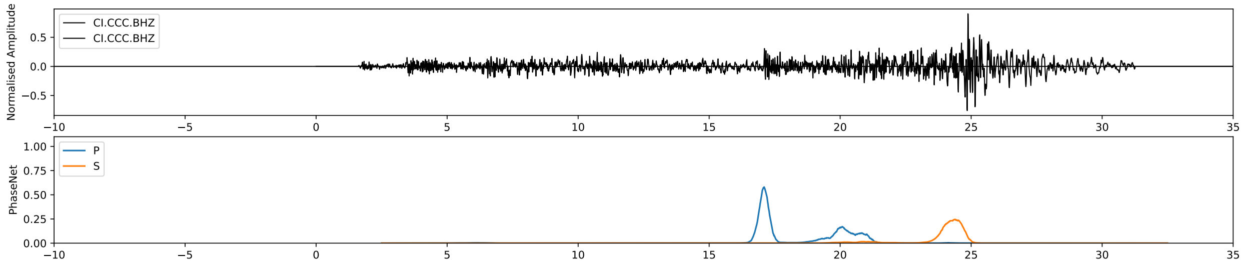


Figure SF4: PhaseNet phase picking results on highly overlapped waveform (30 epm, last row in Fig. SF3, which should have 10 P-phases and 10 S-phases.)

# S3 Experiment details on synthetic dataset

We simulate wave propagation in a region of size 100 km × 100 km × 100 km, with wave speeds ranging from 5km/s to 25km/s in Figs. 6, SF10, SF6 and SF9 to test the association in very extremely complicated scenarios. In Fig. 3, we set the wave speed bounded by 1.5 km/s to 8.5 km/s to compare Harpa with other algorithms in more realistic scenarios.

## S3.1 Known wave speed model

In the known wave speed experiment (Figs. SF2 and SF10), we used the SEG/EAGE 3-D overthrust model [6] (left plot in Fig. SF1), rescaled to our experimental volume. It is remarkable that despite the complexity of the wave speed Harpa achieves near 100% association accuracy, even in the most challenging cases with many overlapping arrivals (green window in Fig. SF2) where the ordinal number of arrivals is completely different from station to station.

## S3.2 Unknown wave speed model

### S3.2.1 Wave speed autoencoders

In Figs. 6, SF6 and SF9, we discretize the wave speed into a 32 × 32 × 32 cube, i.e. $c \in \mathbb{R}^{32\times32\times32}$ (26 × 26 × 26 cube for Fig. 3). We use these cubic images to train a standard CNN autoencoder in `pytorch`. Due to the low-dimensional structure of the dataset, the autoencoder exhibits strong generalization when an appropriate dimension of the latent code $z \in \mathbb{R}^L$ is selected. A large $L$ yields an autoencoder which accurately represents the wave speeds but also leads to slow SGLD inference. In our experiments we tested values of $L$ between 3 and 8. The generalization performance of the autoencoder in the experiment of Fig. 6 is illustrated in Fig. SF5. The encoder comprises three 3D convolutional layers with a kernel size of $3^3$, a stride of 2, and padding of 1, each followed by a ReLU activation function. A subsequent linear layer generates the latent code $z$. Batch normalization is implemented between each layer. The decoder's architecture mirrors that of the encoder.

### S3.2.2 Training the travel time neural field

We compute the travel times from the receivers to to all 32 × 32 × 32 (or 26 × 26 × 26) grid points for the aforementioned 10000 wave speeds using the fast marching method implemented in the `scikit-fmm` package.

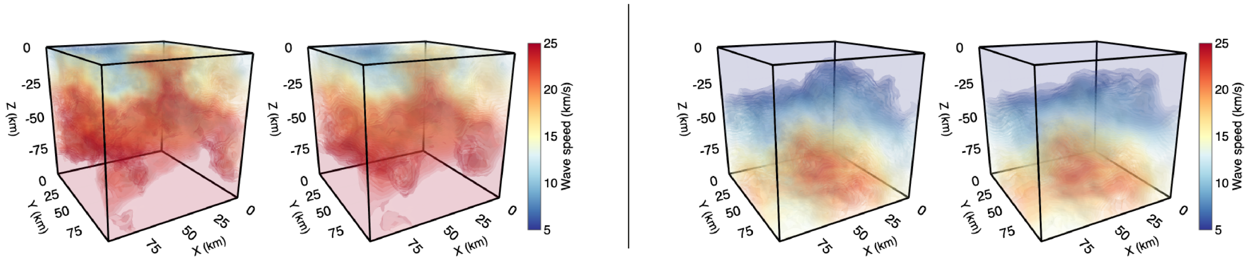


Figure SF5: Two test wave speeds unseen at training time. **Left**: ground truth wave speed model; **Right**: auto-encoder output with $L = 6$.

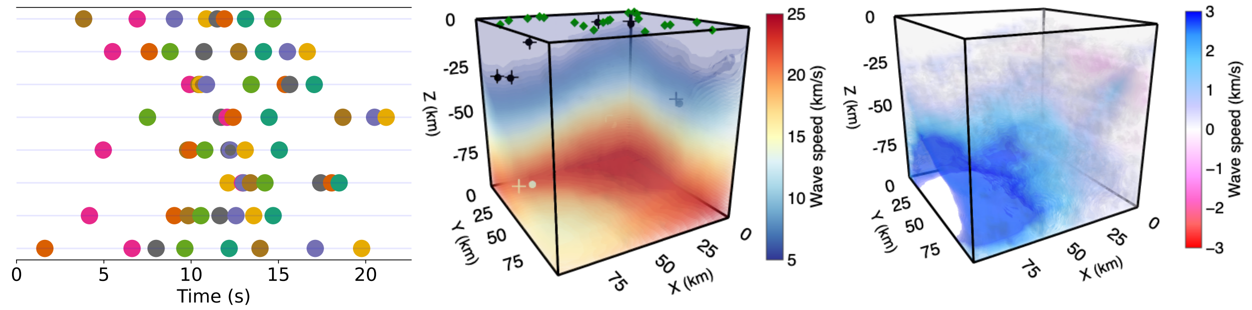


Figure SF6: Association results for 8 sources, 20 stations and $\mathsf{CF} = 0.79$ on Gaussian perturbation dataset. Harpa achieves $\mathsf{ACC} = 96.3\%$ and $e_l = 0.02$. Symbols and encoding are as in Fig. 6.

We create a $(L + 3)$-dimensional feature vector for each grid point by concatenating its coordinate and the corresponding wave speed latent code, which are all scaled in $[0, 1]$ as the input to the neural field. We use a SIREN implicit network, a multilayer perceptron (MLP) with periodic activation functions [7]. The trained SIREN model not only provides accurate predictions of the travel time at the grid points but also immediately yields an interpolation at arbitrary continuous coordinates. The scaling constant $w_0$ in the sinusoidal activation function is important and depends on the grid scaling; we used $w_0 = 15$ or 30.

### S3.2.3 Gaussian random field dataset

In Figs. 6, SF9 and the *OOD* experiment in 3, the wave speeds are samples from the Gaussian random field dataset. To generate this low-dimensional wave speed dataset, we first created 20 three-dimensional Gaussian random fields as basis patterns in which the correlation is determined by the scale-invariant power spectrum $P(k) \sim k^{-\alpha/2}$ [8, 9]. We use $\alpha = 2.5$ in our experiments and rescale the pattern amplitudes to lie between 0 km/s and 15 km/s; representative samples are shown in Fig. SF8. In Figs. 6 and SF9, for each sample, we randomly select up to 3 patterns and then add the selected patterns to a vertical gradient wave speed (Fig. SF7) with weights drawn uniform at random in $[-1, 1]$ and all wave speeds are clipped between 5 km/s and 25 km/s. In Fig. SF5 we show that this dataset is effectively modeled by a 3D convolutional autoencoder. In the *OOD* experiment in Fig. 3, we also randomly select up to 3 patterns, add the selected patterns to a different vertical gradient background (from 3 km/s to 7 km/s, the first wave speed model in Fig. 3), and finally clip them between 1.5 km/s and 8.5 km/s.

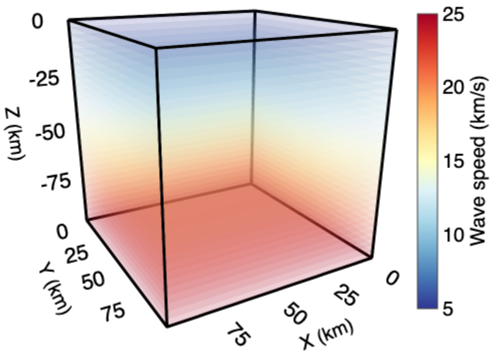


Figure SF7: Vertical gradient wave speed

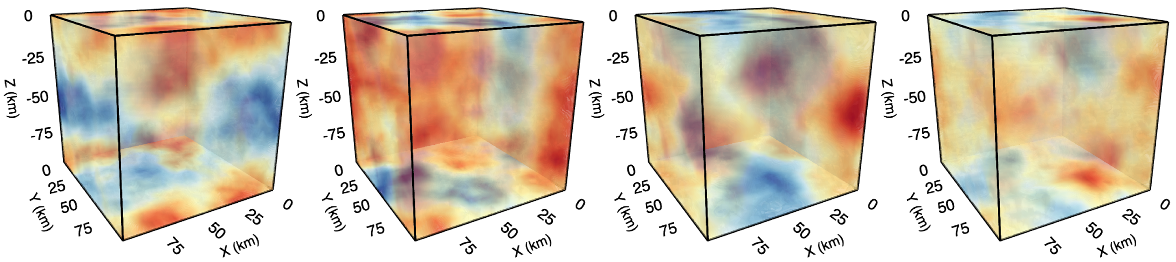

Figure SF8: Four samples of the 3D Gaussian random fields with $\alpha = 2.5$.

### S3.2.4 Gaussian random perturbation dataset

In Figs. 3 and SF6, we report results for a different data set in which we add between one and three random Gaussian perturbations to the vertical gradient wave speed. These perturbations are defined as

$$\Delta c(x, y, z) = A \exp\left(-\frac{1}{2\sigma_x^2}(x - x_0)^2 - \frac{1}{2\sigma_y^2}(y - y_0)^2 - \frac{1}{2\sigma_z^2}(z - z_0)^2\right),$$

where $A$ is drawn uniformly at random from $[-25, 25]$, $x_0, y_0, z_0$ uniformly at random from $[0, 100]$ and $\sigma_x, \sigma_y, \sigma_z$ uniformly at random from $[10, 50]$ in SF6. In Fig. 3, $A$ is drawn uniformly at random from $[1, 15]$, $x_0, y_0, z_0$ uniformly at random from $[0, 100]$ and $\sigma_x, \sigma_y, \sigma_z$ uniformly at random from $[10, 50]$.

### S3.2.5 Distorted and out-of-distribution wave speeds

Next, we study the robustness of the proposed method in situations where the true wave speed comes from a different distribution than the one used to train Harpa's travel time neural field. In other words, the ground truth wave speed is markedly different from any wave speed seen by the autoencoder, both qualitatively and quantitatively.

In the "distortion" experiment (Fig. SF9**a**), we use the same fixed wave speed $c_0$ used in the previous known wave speed experiment to learn travel time neural fields, while the true (test) wave speed is a linear interpolation between $c_0$ and another fixed wave speed $c_1$, $c^* = (1 - p_d)c_0 + p_d c_1$; when $p_d = 0$, there is no model distortion between training and deployment. In the "out of distribution" experiment (Fig. SF9**b**),

we use the travel time neural field for a wave speed distribution described in the previous unknown wave speed experiment. The true (test) wave speed is generated according to $c^* = (1 - p_o)c_2 + p_o c_0$, where $c_2$ is a wave speed randomly sampled in-distribution and $c_0$ is the out-of-distribution perturbation. A large $p_o$ means that $c^*$ is far from the training wave speed distribution In either case we let $c_0$ be the SEG/EAGE 3-D overthrust model, qualitatively rather different from Gaussian random field samples $c_1$ and $c_2$.

We highlight that, compared with the fixed wave speed experiment in Fig. SF9**a**, the generative model in HARPA makes the recovery much more robust. For small CF, the association accuracy (orange heatmap) is still very high even though the test wave speed is far out of distribution. It is further worth noting that in cases where the arrival sequence from different events is similar at all stations (small CF), accurate wave speed recovery and source localization are not necessary for a good association. This observation aligns with previous studies on the low-rate regime where fixed wave speed models which only vary in the depth coordinate yield good association performance.

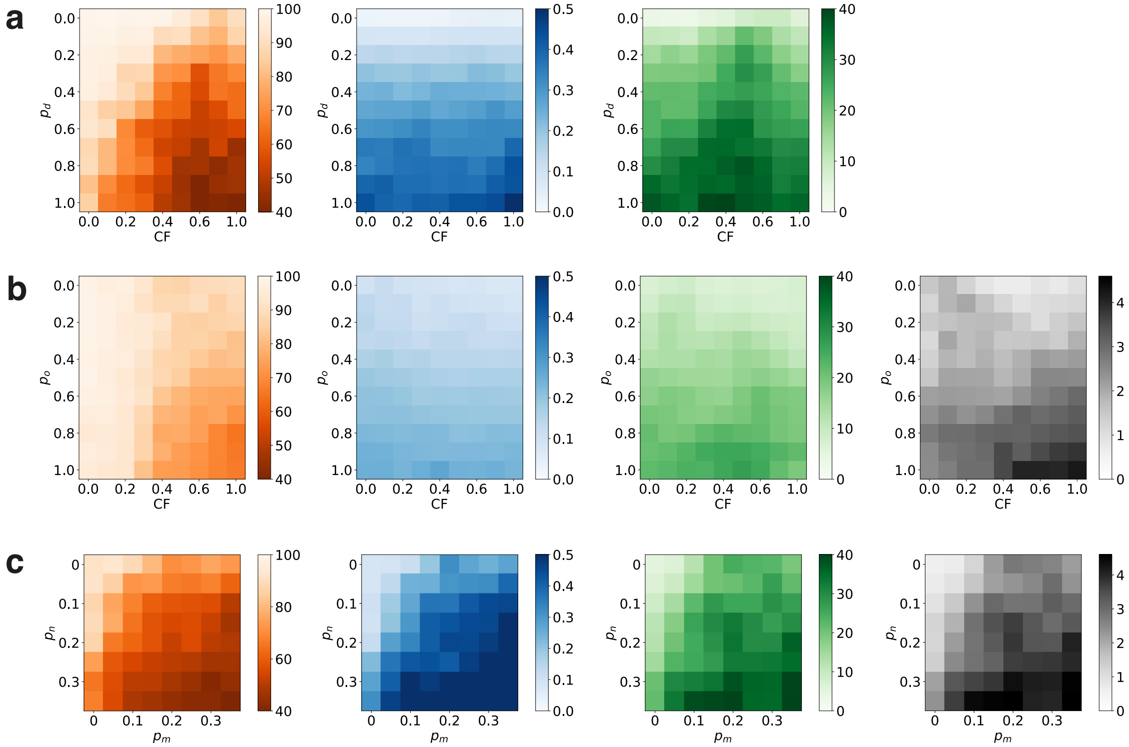


Figure SF9: Robustness of HARPA under distortion and noise quantified by association accuracy ACC (orange), signal matching error $e_l$ in seconds (blue), earthquake location error in km (green) and mean wave speed reconstruction error in km/s (grey), as a function of **(a)** wave speed distortion ($p_d$) and the confusion factor CF; **(b)** excursion from training distribution ($p_o$) and confusion factor CF; **(c)** fraction of noisy ($p_n$) and missing ($p_m$) picks. All values are averages of 20 trials. In **(c)**, the ACC and $e_l$ are determined by comparison with the original noiseless picks and the average CF is 0.80;

### S3.2.6 Spurious and missing picks

When working with real seismograms it may happen that some picks are missing, for example because a station is too far from the source. On the contrary, the peak picking algorithm may make spurious detections. We test the robustness of HARPA to these types of errors. In Fig. SF9**c**, we arbitrarily eliminate a $p_m$ fraction of arrivals at each station and introduce an additional fraction $p_n$ of random picks. When $p_n > p_m$, the number of picks at each station is typically larger than the number of events we are searching for. On the contrary, when $p_n < p_m$, the number of picks at each station is typically smaller than the number of events

we are searching for. We see in the figure that small-to-moderate ratios of noisy and missing picks do not significantly hurt the association accuracy (orange heat map in Fig. SF9**c**) even when CF $= 0.80$.

# S4 Optimization

We use the Python Optimal Transport (POT) package to compute the Wasserstein-2 distance, with $p = 2$. We adopt the RMSProp-preconditioned version of the SGLD [10]. Both the learning rate ($lr$) and the noise factor ($\epsilon$) are selected from $\{10^{-2}, 10^{-3}, 5 \times 10^{-3}, 10^{-4}\}$. The convergence speed depends on the choice of hyperparameters. To manage the exploration-exploitation trade-off, we reduce the learning rate ($lr$) and noise factor to one-tenth of their original value once the loss decreases below a threshold or after 10000 epochs.

In Fig. SF10, we show that due to non-convexity naive (stochastic) gradient descent converges to poor local minima, and that the issue is mitigated by SGLD. We compare SGD and SGLD on the fixed wave speed datasets. To visualize the optimization trajectory, we set the learning rate to 0.005 and $\epsilon = 0.0005$ (cf. (5)) for all epochs. Setting $\epsilon = 0$ reduces SGLD to SGD; the corresponding performance is reported in the second row in Fig. SF10. A visual comparison of the trajectories of the source estimates during optimization (Fig. SF10, right) clearly shows that unlike SGD, SGLD easily escapes bad local minima.

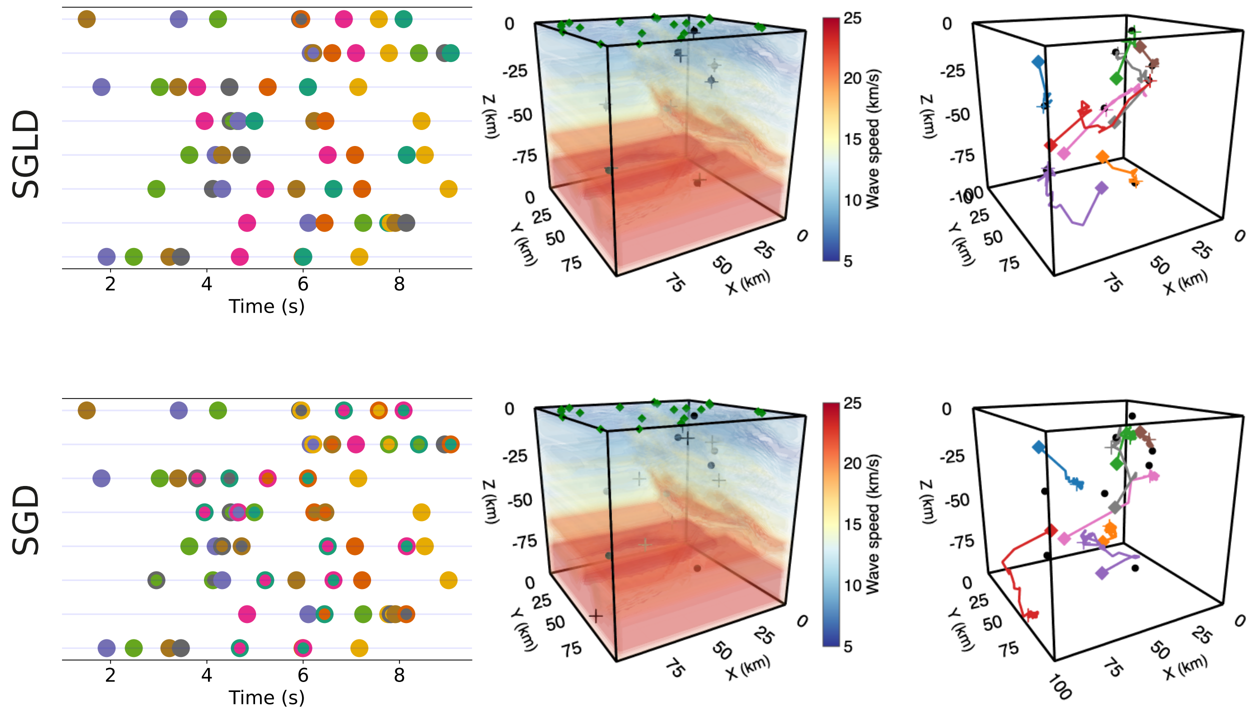


Figure SF10: Association results for 8 sources, 20 stations and CF $= 0.85$ with SEG/EAGE 3-D overthrust model as the known wave speed. **Top row (SGLD)**: ACC $= 92.5\%$, $e_l = 0.02s$. **Bottom row (SGD)**: ACC $= 37.5\%$, $e_l = 0.59s$. Symbols and encoding are as in Fig. 6; the right plot illustrates the source trajectories in the first 30 optimization epochs.

# S5 Real datasets

In the experiment of 2014 Chile (Fig. 4), we test totally 215199 picks (125936 P picks and 89263 S picks) from 20 stations/channels between 2014-03-15 00:00:00 and 2014-04-14 23:59:59 from (`https://github.com/AI4EPS/GaMMA/releases/download/test_data/demo.tar`). For all three algorithms (Harpa, GaMMA, PyOcto), we set the minimum number of picks for a event as 10, and the maximum tolerance of the time of picks as 2 seconds. In Fig. SF11, we also plot the depth v.s. longitude and depth v.s. time of the events detected.

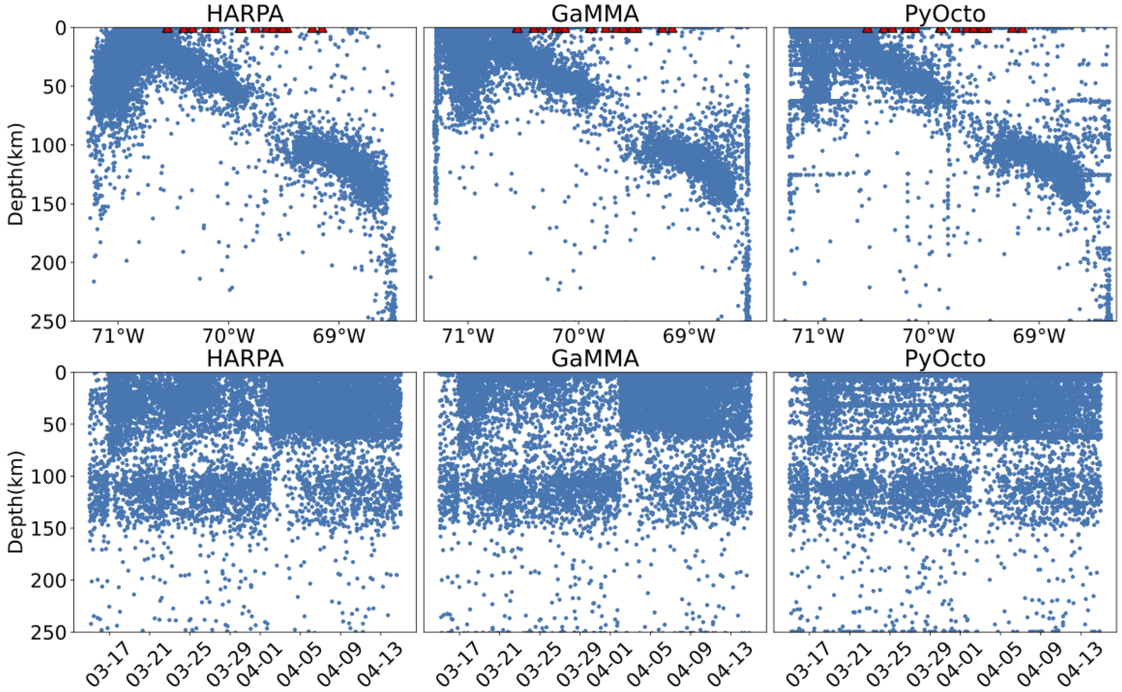


Figure SF11: The events detected 2014 Chile (Fig. 4)

We also applied the generative (unknown) wave speed model in this dataset dataset. The training wave speed dataset is created by augmenting a vertical gradient with 1-3 Gaussian perturbations (similar to Fig. 3 but with different scale). Since 2014 Chile is a very low-frequency sequence, the learnable wave speed did not significantly enhance event detection (as detailed in the main paper). However, we detect significant velocity heterogeneity at depths exceeding 200 km (Fig. SF12). In comparison with existing literature [11], this observation suggests that Harpa partially captures the subducting slab of the oceanic plate.

In the experiment of 2019 Ridgecrest (Fig. SF14), we test totally 78980 picks (38228 P picks and 40752 S picks) from 58 stations/channels between 2019-07-04 17:00:00 and 2019-07-04 23:59:59 also from (`https://github.com/AI4EPS/GaMMA/releases/download/test_data/demo.tar`). For all three algorithms (Harpa, GaMMA, PyOcto), we set the minimum number of picks for one event as 16, the maximum tolerance of the time of picks as 2 seconds. We filter out "noisy" or unreliable events in seismic data based on the proximity of events to stations that detect them. Specifically, we identify the 10 nearest stations to each event. If fewer than 30% of these stations have recorded picks for the event, this event will be deemed unreliable and excluded from further analysis. This filtering approach is also implemented in [12], and an example is provided in the GaMMA project `https://github.com/AI4EPS/GaMMA/blob/master/docs/example_phasenet.ipynb`. Note that in PyOcto, the event locations show stripes. As shown in the documentation of PyOcto, we should increase *location_split_depth* or *location_split_return* to make the locations more accurate. However, when these two parameters increase, PyOcto does not converge within a reasonable time. In Fig. SF14, we also

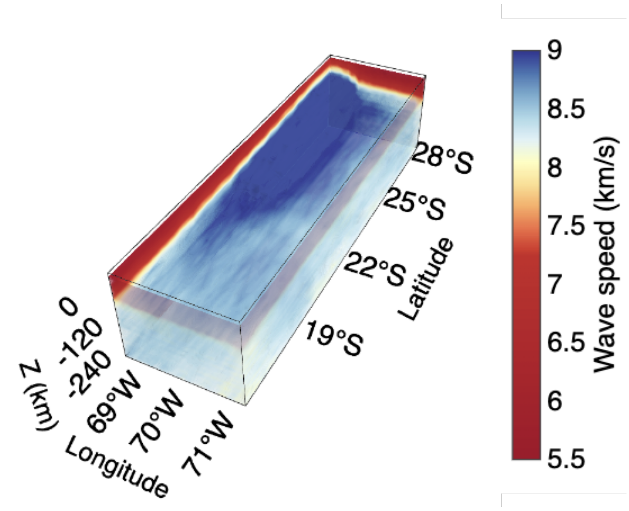


Figure SF12: Recovered wave speed in Chile (Fig. 4)

plot the depth v.s. longitude and depth v.s. time of the events detected in this dataset.

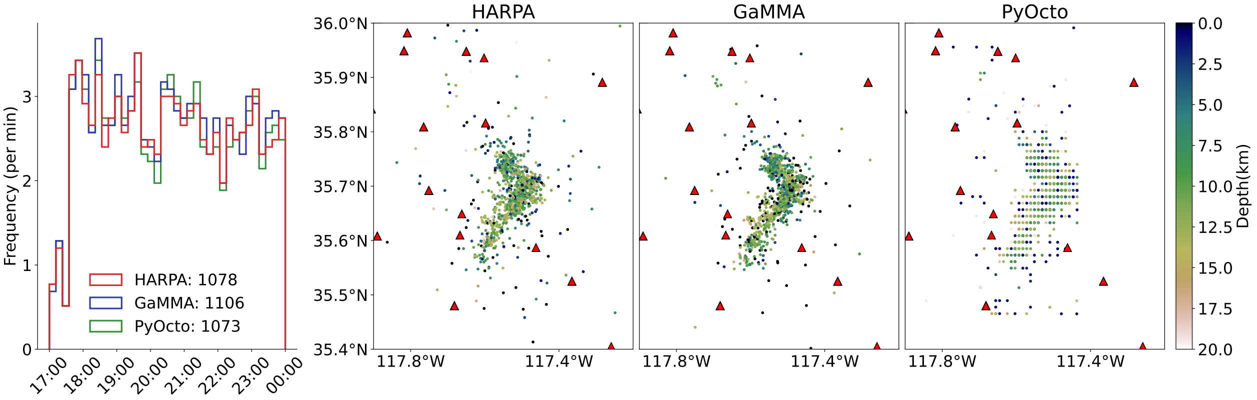


Figure SF13: Performance of Harpa and other algorithms on 2019 Ridgecrest earthquake between 2019-07-04 17:00:00 and 2019-07-04 23:59:59

In the experiment of 2019 Ridgecrest in Fig. 5, we download the waveform from SCEDC in network CI. The picks are labeled by *instance* pretrained PhaseNet in SeisBench[13]. For all three algorithms (Harpa, GaMMA, PyOcto), we set the minimum number of picks for one event as 8 (PhaseNet in SeisBench clusters the arrivals from different channels within the same station, resulting in a smaller number of picks for each event), and the maximum tolerance of the time of picks as 2 seconds.

# S6 Comparison running time

The typical time complexity of a linear sum assignment problem for $M$ events with $N$ stations is $O(NM^3)$. However, since it's common practice to segment a long sequence into shorter windows and process data in parallel (small $M$ for each window), this time complexity does not fully capture the speed advantage of HarpAin high-rate regimes. Inspired by the experiments in the PyOcto paper, we did an analysis of time complexity by documenting the time for event association (Fig. SF15). For very low-rate events, grid-search-based algorithms like REAL and PyOcto are fast. However, for high-frequency events, $\gtrsim$ 30,

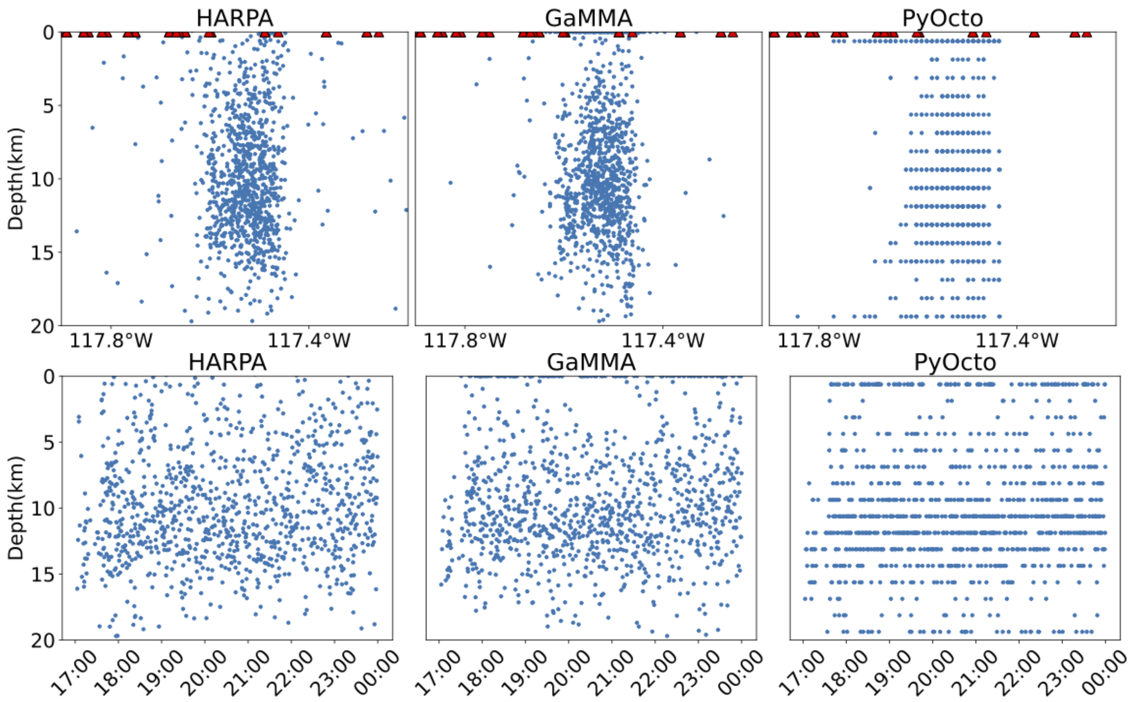


Figure SF14: The events detected 2014 Chile (Fig. 5)

grid-search-based algorithms take significantly longer to converge, while HARPAis much faster as it is less sensitive to event frequency. In Fig. SF15, we show the average time required to assign each event in the experiment where we vary the frequency of the events (in Fig. 1).

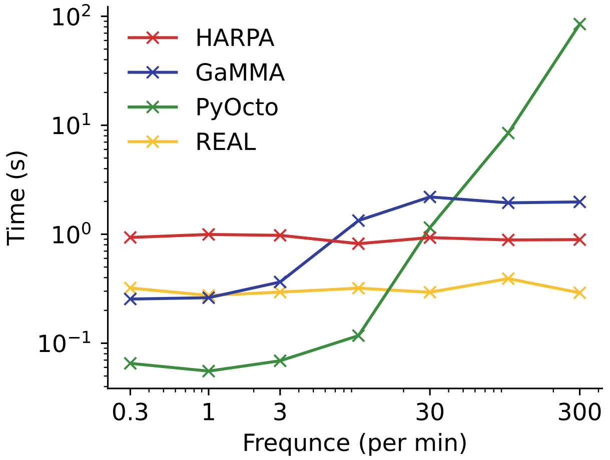


Figure SF15: Average time required to assign each event in the experiment shown in Fig. 1.

## S7 Association and mixed-integer optimization problem

In the main paper, we denote $t_{i,j} = T_c(s_j; r_i) + \tau_j$ as the arrival time of the $j$-th event at the $i$-th station. We can then order these arrivals at this station as $\bar{t}_{i,k} = t_{i,j}$, where $\bar{t}_{i,k}$ denotes the $k$-th observed arrival at this station. The goal of the source–receiver association is to determine which picks correspond to which source ($k$ to $j$). To model this, we define the ground truth association as

$$\alpha^*(k; r_i) := j \leq M,$$

and its corresponding inverse assignment as

$$\alpha^{*-1}(j; r_i) := k \leq M.$$

We aim to infer the assignment $\alpha^*$ (up to a global permutation), the unknown wave speed $c^*$, and the source locations and times $\mathcal{E}^*$, from arrival time data. This can be formulated as the following mixed-integer optimization problem,

$$\underset{\alpha, c, \mathcal{E}}{\text{minimize}} \quad L(\alpha; c, \mathcal{E}), \tag{SE2}$$

where the loss function is defined using a suitable discrepancy metric $\ell(a, b)$ on the arrival times,

$$L(\alpha; c, \mathcal{E}) = \sum_{j \leq M, i \leq N} \ell\left(T_c\left(s_j; r_i\right) + \tau_j,\ \bar{t}_{i,\alpha^{-1}(j; r_i)}\right). \tag{SE3}$$

We mention in the passing that some works deal with the unknown occurrence times by using time difference of arrival (TDoA) data instead of including the takeoff times as optimization variables; this is achieved by minimizing the mismatch loss

$$L^M(\alpha; c, \mathcal{E}) = \sum_{j \leq M, i_a < i_b \leq N} \ell\left(T_c\left(s_j; r_{i_a}\right) - T_c\left(s_j; r_{i_b}\right),\ \bar{t}_{i_a,\alpha^{-1}(j; r_{i_a})} - \bar{t}_{i_b,\alpha^{-1}(j; r_{i_b})}\right). \tag{SE4}$$

To characterize performance we also record the phase association accuracy defined as

$$\mathsf{ACC} = \frac{1}{NM} \sum_{i=1}^{N} \sum_{j=1}^{M} \delta\left(\alpha(j; r_i), \alpha^*(j; r_i)\right) \tag{SE5}$$

where $\delta$ is the Kronecker delta. When the squared difference metric $\ell(a, b) = (a - b)^2$ is used in (SE3), we use $e_l = \sqrt{L(\alpha; c(z), \mathcal{E})/(MN)}$ to characterize the error in arrival time as a consequence of misassociation.

## S8 A Wasserstein misfit for spurious and missing picks

In Eq. (2), we minimize the distance between the observed probability measure and our model probability measure over arrivals as $\text{dist}(\mathbb{Q}, \mathbb{P})$ where dist represents the Wasserstein distance as

$$\text{dist}(\rho_1, \rho_2) = w(\rho_1, \rho_2) = \left(\inf_{\gamma \in \mathcal{C}(\rho_1, \rho_2)} \int |\theta_1 - \theta_2|^p \gamma\left(\mathrm{d}\theta_1,\ \mathrm{d}\theta_2\right)\right)^{1/p}, \tag{SE6}$$

To solve the unbalanced matching, we define a Wasserstein-like mismatch between these arrival sets. We denote the cardinality of a finite set $S$ by $|S|$ and let $\rho_S$ be the uniform probability measure over its elements,$\rho_S = \frac{1}{|S|} \sum_{s \in S} \mathbb{1}_s$. Now, consider two sets of arrival times, $A$ and $B$, which may have different cardinalities. Without loss of generality, assume $|A| \leq |B|$, which accommodates both spurious picks ($K > M$) and missing picks ($K < M$). In this context, the mismatch is defined as the minimal Wasserstein distance $w$ (from Equation (SE6)) over subsets of $B$ with the same cardinality as $A$. Specifically,

$$\widehat{w}(A,B) := \min_{\widetilde{B}\subseteq B,\ |\widetilde{B}|=|A|} w(\rho_A, \rho_{\widetilde{B}}), \tag{SE7}$$

This mismatch can be optimized by sparsity-constrained optimal transport [14]. In fact, in the 1D case it coincides with the loss of the unbalanced linear assignment problem

$$\widehat{w}_p(A,B) = \min_{T\in\mathcal{T}_{|A|,|B|}} \tfrac{1}{|A|}\langle T, C\rangle,$$

where (arbitrarily vectorizing the elements of $A$ and $B$ as $a = (a_1, \dots, a_{|A|})$ and $b = (b_1, \dots, b_{|B|})$) we used

$$\begin{aligned} \mathcal{T}_{|A|,|B|} &:= \left\{ T \in \{0,1\}^{|A|\times|B|} : T\mathbf{1}_{|B|} = \mathbf{1}_{|A|},\ T^\top \mathbf{1}_{|B|} \le \mathbf{1}_{|A|} \right\}, \\ C_{ij} &:= |a_i - b_j|^p. \end{aligned} \tag{SE8}$$

Here $\langle \cdot, \cdot \rangle$ denotes the Frobenius inner product and $T$ the discrete transportation matrix. The all-ones vector of length $K$ is denoted $\mathbf{1}_K$. For vectors $x, y \in \mathbb{R}^K$, the notation $x \le y$ indicates that the inequality holds for all entries.

# References


[1] Weiqiang Zhu and Gregory C Beroza. Phasenet: A deep-neural-network-based seismic arrival-time picking method. *Geophysical Journal International*, 216(1):261–273, 2019.

[2] Weiqiang Zhu, Ian W McBrearty, S Mostafa Mousavi, William L Ellsworth, and Gregory C Beroza. Earthquake phase association using a Bayesian Gaussian mixture model. *Journal of Geophysical Research: Solid Earth*, 127(5):e2021JB023249, 2022.

[3] Maurice G Kendall. A new measure of rank correlation. *Biometrika*, 30(1/2):81–93, 1938.

[4] Zachary E. Ross, Benjamín Idini, Zhe Jia, Oliver L. Stephenson, Minyan Zhong, Xin Wang, Zhongwen Zhan, Mark Simons, Eric J. Fielding, Sang-Ho Yun, Egill Hauksson, Angelyn W. Moore, Zhen Liu, and Jungkyo Jung. Hierarchical interlocked orthogonal faulting in the 2019 Ridgecrest earthquake sequence. *Science*, 366(6463):346–351, 2019.

[5] Zachary E Ross, Weiqiang Zhu, and Kamyar Azizzadenesheli. Neural mixture model association of seismic phases. *arXiv preprint arXiv:2301.02597*, 2023.

[6] Fred Aminzadeh, P Weimer, and T Davis. 3-d salt and overthrust seismic models. *Studies in Geology*, 42:247–256, 1996.

[7] Vincent Sitzmann, Julien Martel, Alexander Bergman, David Lindell, and Gordon Wetzstein. Implicit neural representations with periodic activation functions. *Advances in Neural Information Processing Systems*, 33:7462–7473, 2020.

[8] James M Bardeen, JR Bond, Nick Kaiser, and AS Szalay. The statistics of peaks of Gaussian random fields. *Astrophysical Journal, Part 1 (ISSN 0004-637X), vol. 304, May 1, 1986, p. 15-61. SERC-supported research.*, 304:15–61, 1986.

[9] John Dubinski and RG Carlberg. The structure of cold dark matter halos. *Astrophysical Journal, Part 1 (ISSN 0004-637X), vol. 378, Sept. 10, 1991, p. 496-503.*, 378:496–503, 1991.

[10] Chunyuan Li, Changyou Chen, David Carlson, and Lawrence Carin. Preconditioned stochastic gradient Langevin dynamics for deep neural networks. In *Proceedings of the AAAI Conference on Artificial Intelligence*, volume 30, 2016.

[11] Caio Ciardelli, Marcelo Assumpção, Ebru Bozdağ, and Suzan van der Lee. Adjoint waveform tomography of south america. *Journal of Geophysical Research: Solid Earth*, 127(2):e2021JB022575, 2022.

[12] Miao Zhang, William L Ellsworth, and Gregory C Beroza. Rapid earthquake association and location. *Seismological Research Letters*, 90(6):2276–2284, 2019.

[13] Jack Woollam, Jannes Münchmeyer, Frederik Tilmann, Andreas Rietbrock, Dietrich Lange, Thomas Bornstein, Tobias Diehl, Carlo Giunchi, Florian Haslinger, Dario Jozinović, et al. Seisbench—a toolbox for machine learning in seismology. *Seismological Society of America*, 93(3):1695–1709, 2022.

[14] Tianlin Liu, Joan Puigcerver, and Mathieu Blondel. Sparsity-constrained optimal transport. In *International Conference on Learning Representations*, 2023.
